# Supplementary material for: Thermal hysteresis and the heat shuttling effect
Source: arXiv:2302.09100 ancillary file (2023-02-17)
Supplement: Supplementary file 1 [file Shuttling_Hysteresis_SUPPLEMENTARY_230216.pdf]

# Supplementary material
# Thermal hysteresis and the heat shuttling effect

Jean-Claude Krapez
*ONERA, The French Aerospace Lab, DOTA, F-13661 Salon cedex Air, France*
(*Electronic mail: jean-claude.krapez@onera.fr)

## I. PRESENTATION

For the sake of clarity and completeness, here we provide some details on the numerical model that was developed to calculate the temperature evolution in a PCM layer with hysteresis, and on the verification performed against an analytical model for the limiting case of a linear material. We also describe the link between a series of six animations provided in mp4 format showing the dynamic evolution of joint temperature and conductivity distributions and the corresponding figures in the main text.

## II. NUMERICAL MODEL

We assume 1D heat diffusion along a layer of thickness $l$ which is in perfect contact with two heat baths, where the left one is at a sinusoidally modulated temperature:

$$T_L(t) = T_c + T_a \sin(2\pi f t), \tag{1}$$

and the right one either at constant temperature:

$$T_R(t) = T_c, \tag{2}$$

or equally modulated but with a phase lag:

$$T_R(t) = T_c + T_a \sin(\max(0; 2\pi f t - \delta)). \tag{3}$$

The heat equation to solve is:

$$\rho \frac{\partial H(T(x,t))}{\partial t} = -\frac{\partial}{\partial x}(\varphi(x,t)), \tag{4a}$$

with the heat-conduction flux $\varphi(x,t)$ defined by:

$$\varphi(x,t) = -k(T(x,t)) \frac{\partial T(x,t)}{\partial x}. \tag{4b}$$

### A. General equations for the discretized fields

The numerical solution is obtained after discretizing in space and applying the well known finite volume approach. For simplicity we used a constant space discretization interval $\Delta x = l/M$ where $M$ is the number of cells; we also applied the explicit (Euler) time marching method which, from the temperature, enthalpy and conductivity discretized fields known at time step $n$ allows expressing the enthalpy field at time step $n+1$ according to:

$$\rho \frac{H_i^{n+1} - H_i^n}{\Delta t} = \frac{\varphi_{i-1/2}^n - \varphi_{i+1/2}^n}{\Delta x}, \tag{5a}$$

$$\varphi_{i-1/2}^n = -k_{i-1/2}^n \frac{T_i^n - T_{i-1}^n}{\Delta x}, \tag{5b}$$

$$\varphi_{i+1/2}^n = -k_{i+1/2}^n \frac{T_{i+1}^n - T_i^n}{\Delta x}, \tag{5c}$$

where the subscripts $i$, $i-1$, and $i+1$ are affected to temperature and enthalpy to designate the mean temperature, resp. enthalpy, of the cells numbered $i$, $i-1$, and $i+1$ of common thickness $\Delta x$, whereas the subscripts $i-1/2$ and $i+1/2$ are affected to heat flux and conductivity to designate the heat flux and conductivity at the left, resp. right boundary of the cell $i$. The conductivity at these boundaries is calculated according to the rule of thermal resistances in series, based on resp. the mean conductivity of cells $i-1$ and $i$ on one side and of the cells $i$ and $i+1$ on the other side. :

$$k_{i-1/2}^n = \frac{2}{\frac{1}{k_{i-1}^n} + \frac{1}{k_i^n}}, \tag{6a}$$

$$k_{i+1/2}^n = \frac{2}{\frac{1}{k_i^n} + \frac{1}{k_{i+1}^n}}, \tag{6b}$$

where $k_{i-1}^n$, $k_i^n$ and $k_{i+1}^n$ are the conductivity values inferred from the mean temperature of the cells $i-1$, $i$, and $i+1$ (see §II E for their determination).

### B. Equations for the flux at the boundaries

The relations in 5(b) and (c) giving the flux at cell boundaries are valid except for the two boundaries of the domain (PCM layer). There are two boundary conditions of 1$^{st}$ type (Dirichlet) on both sides of the domain. The flux at the left boundary is thus expressed based on the Taylor expansions of the temperature at the center of first and second cells with respect to the temperature at the left side of the leftmost cell. A weighted difference of these two expansions allows eliminating the second order terms, which yields an expression for the temperature derivative at the left boundary which is of order $O(\Delta x^3)$. Hence, the flux at the left boundary is expressed as:

$$\varphi_{1/2}^n = k_{1/2}^n \frac{9T_1^n - 8T_{1/2}^n - T_2^n}{3\Delta x}, \tag{7}$$

where the subscript $1/2$ refers to the left side of the leftmost cell. A symmetrical operation is performed to get the flux at the right boundary of the domain as a function of the temperature of cell $M-1$, cell $M$, and of the temperature on the right

side of cell $M$:

$$\varphi^n_{M+1/2} = k^n_{M+1/2} \frac{-9T^n_M + 8T^n_{M+1/2} + T^n_{M-1}}{3\Delta x}, \quad (8)$$

where the subscript $M+1/2$ refers to the right side of the rightmost cell.

### C. Initialization

The initial boundary temperatures, $T^0_{1/2}$ and $T^0_{M+1/2}$, are those specified by the boundary conditions in Eq. (1)-(2) or (12)-(13) in the main text, at time $t=0$, i.e. $T^0_{1/2} = T_L(t=0)$ and $T^0_{M+1/2} = T_R(t=0)$. They share a common value, $T_L(t=0) = T_R(t=0) = T_c$. Two scenarios were envisioned in this paper, either the thermal baths have previously reached this value by heating (from below 333 K) or by cooling (from above 345 K). Any point of the PCM then reaches (asymptotically) the same uniform equilibrium temperature $T_c$. This isothermal state is considered to be the one at $t=0$. The conductivity is then the same everywhere at $t=0$, the value of which is calculated from Eq. (3)-(4) in the main text, with reference to the heating or cooling curve of the main hysteresis loop in Fig. 2(a) depending on whether the common value $T_c$ has been reached by heating or cooling the heat baths. Enthalpy as well is uniform at $t=0$, the value of which is obtained from Eq. (3) and (5) in the main text, by referring to the appropriate heating curve or cooling curve in Fig. 2(b).

### D. Temperature determination from the enthalpy

The enthalpy increment $H^{n+1}_i - H^n_i$ is evaluated at each time step and for each cell $i = 1, M$ by applying Eq. 5(a). Two virtual temperatures are then calculated. The first one, $T^{v,S}$, is based on the assumption that the enthalpy variation is assimilated to sensible heat:

$$T^{v,S} = T^n_i + \frac{H^{n+1}_i - H^n_i}{C}, \quad (9)$$

where $C$ is the specific heat (assumed equal and constant for both isolating and metallic phases in the small temperature range considered). The second one, $T^{v,L}$, is obtained by inverting the enthalpy value $H^{n+1}_i$ into temperature according to Eq. (6)-(9) in the main text. This means inverting the enthalpy value into temperature according to the heating or cooling curve in Fig. 2(b). The selection between the heating and cooling curves, and correspondingly the limiting joint values $H_i$ and $H_m$ in Eq. (6)-(9) in the main text, is made depending on the sign of the enthalpy variation $H^{n+1}_i - H^n_i$. If it is positive, we refer to the heating curve, and if it is negative, to the cooling curve. Then, if the enthalpy variation is positive, the new cell temperature is set to:

$$T^{n+1}_i = \min\left(T^{v,S}, T^{v,L}\right). \quad (10)$$

Alternatively, if it is negative, the new cell temperature is set to:

$$T^{n+1}_i = \max\left(T^{v,S}, T^{v,L}\right). \quad (11)$$

### E. Conductivity determination from the temperature

Once the temperature field at time step $n+1$ has been evaluated, $T^{n+1}_i$, $i = 1, M$, together with the boundary values $T^{n+1}_{1/2} = T_L(t = t_{n+1})$ and $T^{n+1}_{M+1/2} = T_R(t = t_{n+1})$, one has to calculate the corresponding conductivity values, namely $k^{n+1}_i$, $i = 1, M$, in addition to $k^{n+1}_{1/2}$ and $k^{n+1}_{M+1/2}$. For each of these $M+2$ temperature values, a virtual conductivity $k^v$ is first calculated based either on the heating curve or the cooling curve of the main hysteresis loop in Fig. 2(a), depending on whether the temperature has increased or decreased from time step $n$ to time step $n+1$. This amounts to use Eq. (4) in the main text, with the volume fraction of the metallic domains evaluated with Eq. (3) in the main text, which is fed with the proper values of the temperature-transition limits $T_i$ and $T_m$ (i.e. by referring to the due heating or cooling process). Then, if the temperature has increased from time step $n$ to time step $n+1$, the new conductivity is obtained from:

$$k^{n+1}_i = \max\left(k^n_i, k^v\right); \; i = 1/2, 1, 2 ... M-1, M, M+1/2, \quad (12)$$

whereas if it has decreased, the new conductivity is obtained from:

$$k^{n+1}_i = \min\left(k^n_i, k^v\right); \; i = 1/2, 1, 2 ... M-1, M, M+1/2. \quad (13)$$

### F. Time step, space discretization, and convergence criteria

The time step is based on the stability criterion related to the explicit (Euler) scheme when applied to a domain with uniform diffusivity $a$, which reads:

$$\Delta t \leq \Delta t_{max} = \frac{\Delta x^2}{2a}. \quad (14)$$

In the present case of a time-varying diffusivity field bounded by the diffusivity values of the isolating phase, $a_i = 1.09$ mm$^2$ s$^{-1}$, and the metallic phase, $a_m = 1.81$ mm$^2$ s$^{-1}$, we adopted a conservative rule by considering the highest possible diffusivity with, in addition, a safety factor of $1/2$:

$$\Delta t = \frac{1}{2} \frac{\Delta x^2}{2a_m}. \quad (15)$$

Actually, the largest integer divider of the time period smaller than the previous value was finally selected for $\Delta t$. The number of time steps in one period is then called $N$. The simulations lasted over several periods until reaching the stationary periodic regime with sufficient accuracy. Once the $J$-th period ended, the temperature distribution $T^{JN}_i$ was compared with the one obtained one period before, i.e. $T^{(J-1)N}_i$, to provide the RMS error $E_T$:

$$E_T = \left( \frac{1}{M} \sum_{i=1}^{i=M} (T^{JN}_i - T^{(J-1)N}_i)^2 \right)^{1/2}. \quad (16)$$

On the other side, the flux was averaged over the last period to give:

$$\overline{\varphi_i} = \frac{1}{N} \sum_{n=(J-1)N+1}^{n=JN} \varphi_i^n \,;\; i = 1,...,M. \tag{17}$$

Then, the time-mean of the flux was also averaged over space to give:

$$\overline{\overline{\varphi}} = \frac{1}{M} \sum_{i=1}^{i=M} \overline{\varphi_i}, \tag{18}$$

which corresponds to the net heat flux discussed in the main text and was written there as $\overline{\varphi(t)}$.

In the stationary periodic regime, the time-mean of the flux, $\overline{\varphi_i}$, should be uniform, also, the residual (relative) error on the net heat flux, $E_{\overline{\varphi(t)}}$ was defined as:

$$E_{\overline{\varphi(t)}} = \frac{\max\left(\overline{\varphi_i}\right) - \min\left(\overline{\varphi_i}\right)}{\max\left(1, |\overline{\overline{\varphi}}|\right)}. \tag{19}$$

The stopping criterion was the joint satisfaction of $E_T < 10^{-4}K$ and $E_{\overline{\varphi(t)}} < 10^{-3}$. Depending on the thermal conditions, this was reached in about four to several tens of periods (up to 100 in some cases).

The PLM material was discretized into $M$ cells of equal thickness $\Delta x$. Depending on the modulation frequency, different values for $M$ were tested: 29, 53, 105, 165 and 205. One of these values was retained if, when comparing the net heat flux calculated with this value and with the value before in the former list, the relative difference was less than $4 \cdot 10^{-3}$. Also, for frequencies up to $f = 0.3$ Hz (this frequency value was considered for most numerical applications in the main text), a number of $M = 53$ cells was retained. Then, for frequencies up to $f = 10$ Hz, 30 Hz, and 100 Hz, $M = 105$ cells were used, resp. 165 and 205.

## III. MODEL VERIFICATION

A simple verification was made against an analytical model describing the case of a linear material submitted to the same boundary conditions, namely a fixed temperature $T_c$ at the right boundary and a modulated temperature of amplitude $T_a$ at the left boundary and same mean temperature $T_c$. For this purpose, we selected for the input data of the numerical model: $T_c = 350$ K and $T_a = 1$ K. As a consequence, the PCM remains constantly and totally in the metallic phase.

The relation between the Fourier transforms of the temperature ($\Theta_L$ and $\Theta_R$) and of the heat flux ($\Phi_L$ and $\Phi_R$) at the left and right boundaries is given by the quadrupole expression:

$$\begin{bmatrix} \Theta_L \\ \Phi_L \end{bmatrix} = \boldsymbol{M} \begin{bmatrix} \Theta_R \\ \Phi_R \end{bmatrix} \quad ; \quad \boldsymbol{M} = \begin{bmatrix} A & B \\ C & D \end{bmatrix}, \tag{20}$$

where

$$\begin{aligned} A =& D = \cosh\left(\xi\sqrt{i\omega}\right), \\ B =& \frac{1}{b\sqrt{i\omega}} \sinh\left(\xi\sqrt{i\omega}\right), \\ C =& b\sqrt{i\omega} \sinh\left(\xi\sqrt{i\omega}\right), \end{aligned} \tag{21}$$

where $b$ is the thermal effusivity of the material, $b = \sqrt{k\rho C}$, and $\xi$ is the square root of the diffusion time through the total thickness $l$, namely $\xi = l/\sqrt{a}$. The product $\xi\sqrt{i\omega}$ can also be expressed as $\alpha(1+i)$ with $\alpha = l/\mu$ where $\mu$ is the thermal penetration depth, $\mu = \sqrt{2a/\omega}$. Knowing that $\Theta_R = 0$, the Fourier transform of the heat flux at the left and right boundaries is then obtained as:

$$\Phi_L = b\sqrt{i\omega}\Theta_L \frac{\cosh\left(\xi\sqrt{i\omega}\right)}{\sinh\left(\xi\sqrt{i\omega}\right)} \,;\; \Phi_R = b\sqrt{i\omega}\Theta_L \frac{1}{\sinh\left(\xi\sqrt{i\omega}\right)}. \tag{22}$$

The verification focused on the heat flux on the left boundary. After some algebraic manipulations, we easily find that the amplitude $|\Phi_L|$ is expressed by:

$$|\Phi_L| = \frac{k\sqrt{2}|\Theta_L|}{\mu} \left(\frac{1+\tan^2(\alpha)\tanh^2(\alpha)}{\tan^2(\alpha)+\tanh^2(\alpha)}\right)^{1/2} \tag{23}$$

and the phase, noted $P(\Phi_L)$, is expressed by:

$$P(\Phi_L) = \frac{\pi}{4} + \arctan\left(\frac{\tan(\alpha)\left(\tanh^2(\alpha)-1\right)}{\tanh(\alpha)\left(\tan^2(\alpha)+1\right)}\right). \tag{24}$$

When $\alpha \to \infty$ (thermally thick material), we retrieve asymptotically the solution of a semi-infinite medium; in particular, the heat flux sinusoidal modulation is $\pi/4$ ahead of that of temperature.

A comparison between the heat flux values obtained with the analytical solution and the numerical model over one period has shown a relative RMS error of $9 \cdot 10^{-6}$ and a maximum relative error of $1.5 \cdot 10^{-5}$ (the differences were normalized by the maximum value of the theoretical flux), which was deemed satisfactory.

## IV. ANIMATIONS

Animations are provided that complement the figures 3, 5, and 11 in the main text. These figures represent the combined temperature and conductivity distributions inside the $VO_2$ layer at four particular times during a period $P$ of the stationary cycling (namely at $t = P/4,\ P/2,\ 3P/4,\ P$). The animations describe fluently the time evolution of these distributions (the time step of the recording was 0.5° of phase). The correspondance between the animations and the figures is described in the following table. Refer to the captions of the figures in the main text for an explanation of the conditions of the PCM thermal simulation.

TABLE I. Correspondance between the animations (mp4 format) and the figures in the main text.

| Figure | Animation |
|---|---|
| 3(a) | animation-fig-3a |
| 3(b) | animation-fig-3b |
| 5(a) | animation-fig-5a |
| 5(b) | animation-fig-5b |
| 11(a) | animation-fig-11a |
| 11(b) | animation-fig-11b |
